# Supplementary material for: Quantum frequency conversion to telecom of single photons from a nitrogen-vacancy center in diamond
Source: arXiv:1801.03304 ancillary file (2018-06-22)
Supplement: Supplementary file 1 [file Qtelecom_SI_article_final.pdf]

# Supplemental Material
# Quantum frequency conversion to telecom of single photons from a nitrogen-vacancy center in diamond

Anaïs Dréau[1,2,3], Anna Tcheborateva[1,4], Aboubakr El Mahdaoui[1,2], Cristian Bonato[1,2], and Ronald Hanson[1,2]
[1] *QuTech, Delft University of Technology, P.O. Box 5046, 2600 GA Delft, The Netherlands*
[2] *Kavli Institute of Nanoscience, Delft University of Technology, P.O. Box 5046, 2600 GA Delft, The Netherlands*
[3] *Laboratoire Charles Coulomb, Université de Montpellier and CNRS, 34095 Montpellier, France and*
[4] *Netherlands Organisation for Applied Scientific Research (TNO), P.O. Box 155, 2600 AD Delft, The Netherlands*

## I. PPLN WAVEGUIDE CHARACTERISTICS

Before running the frequency conversion experiment with NV center single photons, we investigated the performances of the different waveguides (WG) of the PPLN crystal to pick the one having the best tradeoff between high conversion efficiency and low noise. The PPLN crystal consists of 12 waveguides, split into 6 families; each family being associated with a given quasi-phase-matching (QPM) grating.

The conversion efficiency was measured classically in free space by using a CW laser operating at 637 nm and measuring the down-converted light power on a powermeter installed before the single-mode fiber (see Fig. 1 main text). The results are depicted for 4 different waveguides on Figure 1 (a). The noise produced by the pump beam was recorded on the SSPD at the end of the down-conversion stage and in continuous excitation while blocking the red beam (Fig. 1 (b)). Both the conversion efficiency and the noise resulting from the pump interaction with the non-linear crystal is waveguide dependent. Surprisingly, the evolution of noise counts with pump power deviates from the proportional relationship that was observed on both Stokes Raman scattering [1] and SPDC noise [2]. So far, we do not understand this discrepancy. We chose WG3 to perform the quantum frequency conversion as it reaches the maximum conversion efficiency for the lowest input pump power. (Note that the conversion efficiency achieved with WG3 was further improved to obtain the data depicted on Figure 3(b) of the article.) Its QPM curve displayed on Figure 1 (c) was measured in free space and by tuning the crystal temperature. The deviation from the theoretical cardinal sinus curve for perfect QPM indicates imperfections in the fabrication errors in the poling periods of the PPLN crystal [3].

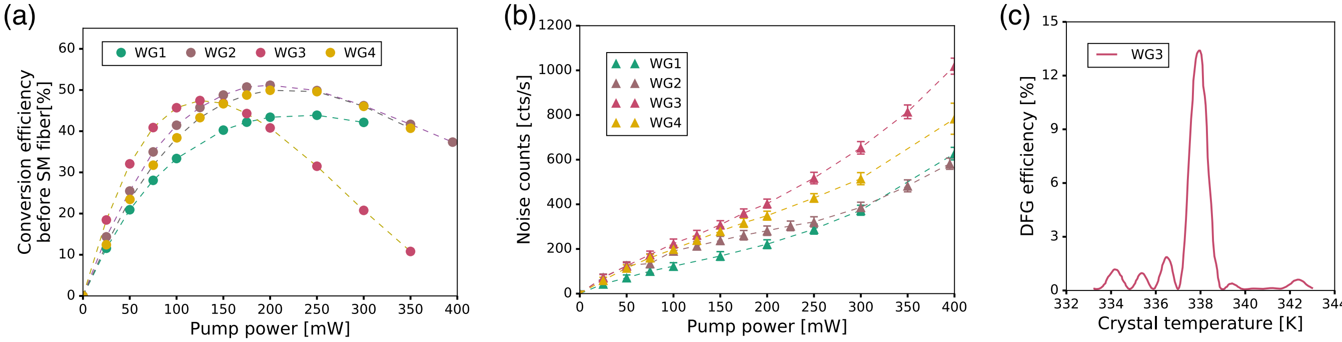


FIG. 1. Evolution of the (a) classical conversion efficiency and the (b) pump-induced noise counts with increasing the input pump power for four different waveguides. (c) Quasi-phase-matching curve of WG3 obtained by tuning the PPLN crystal temperature.

## II. AUTOCORRELATION FUNCTION $g^{(2)}(\tau)$ FOR PULSED HBT EXPERIMENT

In contrast to off-resonant excitation, continuous resonance excitation of an NV centre leads to bleaching due to spin flips, spectral diffusion or ionization to the neutral charge state [4]. To limit the occurence of those random processes, the number of resonant optical $\pi$-pulses per sequence was restrained to 15. After each sequence, the NV's spin was initialized by optical pumping. The sequence was repeated 250 times before verifying that the NV center

was still in the negative charge state and that the associated optical transition was resonant with the excitation laser. More details about the general sequence can be found in [4].

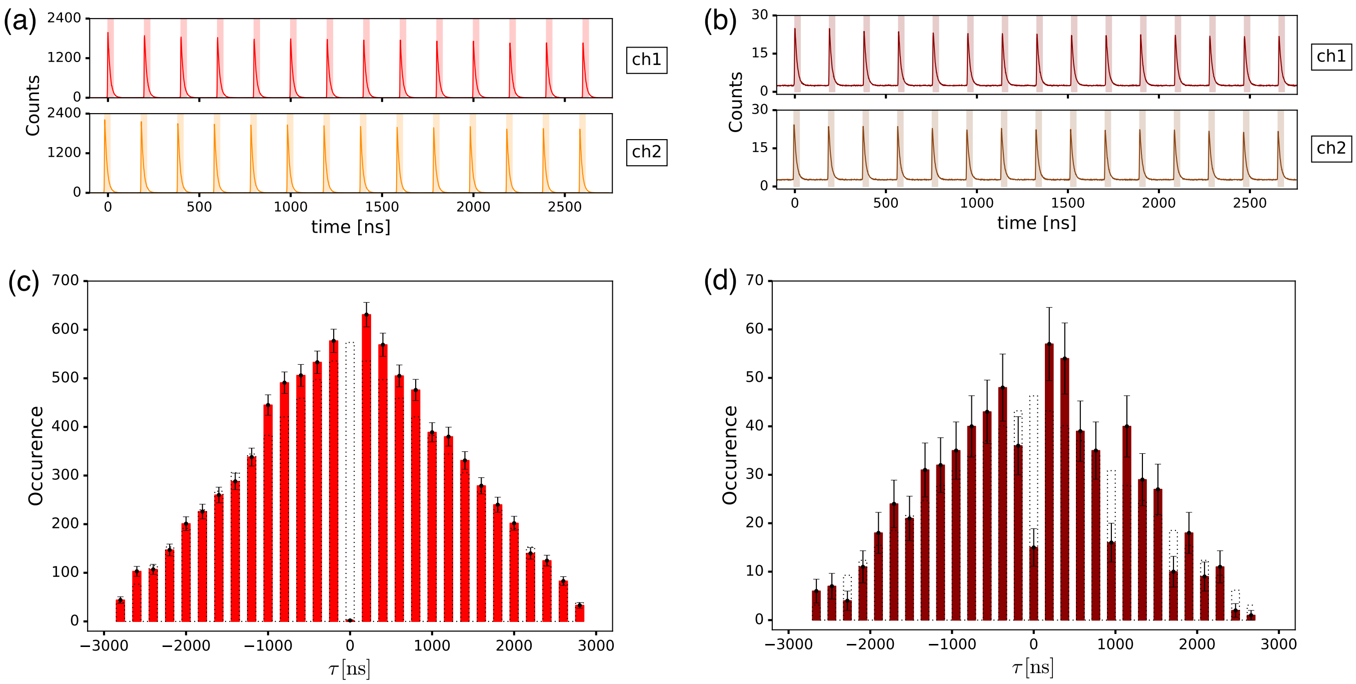


FIG. 2. Count histograms recorded on the two detector channels (a) before and (b) after frequency conversion of the NV center single photons. The shaded areas represent the filtering time windows to select out the counts. (c)-(d) Respective resulting coincidence delay histograms. The dash bars represent the expected coincidence counts for a coherent state having the same intensity as the NV center photon beam. The error bars correspond to one standard deviation assuming Poisson counting statistics.

The count histograms showing the NV center response to the 15 excitation pulses are displayed for both channels on Figures 2(a) and (b) respectively before and after frequency conversion. We filtered out the clicks in a 25-ns time windows following the beginning of each optical excitation (see Figure 2(a) and(b)). Figures 2 (c) and (d) show the histograms of the time delay between coincidence clicks occurring on the two channels during the same sequence, respectively before and after down-conversion. They exhibit pyramidal shape with $2\times15-1 = 29$ coincidence windows due to the finite number of temporal windows. To obtain the second-order autocorrelation function of the input field $g^{(2)}(\tau)$, the coincidence histograms have to be divided by the number of coincidence counts one would get if the input single photons were replaced by a coherent classical state having the same intensity [5]. The normalization coefficient for each coincidence window $i \in [\![-15; 15]\!]$ can be calculated by the formula :

$$K^{(i)}_{norm} = (15 - |i|) \cdot p^{(1)}_c \cdot p^{(2)}_c \cdot N_{rep} \tag{1}$$

where $p^{(1)}_c$ and $p^{(2)}_c$ are respectively the mean counts detected per optical window on channels 1 and 2, and $N_{rep}$ is the number of sequence repetitions. The value of those coefficients are indicated on each coincidence histogram by the dash bars. The outer bars of the coincidence count histogram, corresponding to long delay times for which the detections of photons should not be correlated anymore, match well the values expected for the coherent state as input. In other words, this would lead to $g^{(2)}(|\tau| > 1\mu s) \approx 1$, indicating that the normalization of the coincidence histogram is correct. The $g^{(2)}(\tau)$ displayed on Figures 1 (a) and (b) of the article represent a zoom-in into in the central coincidence time windows.

[1] Sebastian Zaske, Andreas Lenhard, and Christoph Becher, "Efficient frequency downconversion at the single photon level from the red spectral range to the telecommunications C-band," Optics Express **19**, 12825–12836 (2011).

[2] J. S. Pelc, C. Langrock, Q. Zhang, and M. M. Fejer, "Influence of domain disorder on parametric noise in quasi-phase-matched quantum frequency converters," Optics Letters **35**, 2804–2806 (2010).

[3] M. M. Fejer, G. A. Magel, D. H. Jundt, and R. L. Byer, "Quasi-phase-matched second harmonic generation: tuning and tolerances," IEEE Journal of Quantum Electronics **28**, 2631–2654 (1992).

[4] H. Bernien, B. Hensen, W. Pfaff, G. Koolstra, M. S. Blok, L. Robledo, T. H. Taminiau, M. Markham, D. J. Twitchen, L. Childress, and R. Hanson, "Heralded entanglement between solid-state qubits separated by three metres," Nature **497**, 86–90 (2013).

[5] A. Beveratos, S. Kühn, R. Brouri, T. Gacoin, J.-P. Poizat, and P. Grangier, "Room temperature stable single-photon source," The European Physical Journal D **18**, 191–196 (2002).
